# Supplementary material for: Retrieval-Seeded Diffusion for Semantic Flow Models
Source: arXiv:2611.39943 source file (2026-11-29)
Supplement: Supplementary file 1 [file fig_div_keff_supp.tex]

\begin{figure}[b]%
  \centering
  \input{figures/div_keff/values}%
  \input{figures/div_keff/style}%
  \ifdefined\figcachebegin\figcachebegin{div_keff_supp}\fi
  \dklegend{3}{\addlegendimage{dk base}\addlegendentry{Released sampler}
    \addlegendimage{dk lpips}\addlegendentry{LPIPS}
    \addlegendimage{dk vendi}\addlegendentry{Vendi}}
  \\[1pt]
  \dkpanel{rae}{dkdiv}{ylabel={LPIPS $\uparrow$ (\%)}, ymin=-14, ymax=8, ytick={-10,-5,0,5}}{\dkplot{rae}{lpips}}{}{$\tau = 0.02$}\hfill
  \dkpanel{rae}{dkdiv}{ylabel={Vendi $\uparrow$ (\%)}, ymin=-14, ymax=8, ytick={-10,-5,0,5}}{\dkplot{rae}{vendi}}{}{$\tau = 0.02$}
  \ifdefined\figcacheend\figcacheend\fi
  \caption{\textbf{LPIPS and Vendi against the effective number of neighbours.} The other two diversity
    measures of \cref{fig:div_keff}, for \method on Scale-RAE, each as the change
    from the released sampler (dashed). Both rise with $k_\mathrm{eff}$, as DreamSim does. The dotted line marks
    our $\tau = 0.02$.}
  \label{fig:div_keff_supp}
\end{figure}
