# Supplementary material for: Retrieval-Seeded Diffusion for Semantic Flow Models
Source: arXiv:2611.39943 source file (2026-11-29)
Supplement: Supplementary file 2 [file fig_supp_qual_art_anime.tex]

\input{figures/supp_qual/values}%
\begin{figure*}[p]%
  \begin{minipage}[t][0.995\textheight][s]{\textwidth}
  \centering
  \input{figures/supp_qual/layout}%
  \qheadrow
  \qrow{art}{rae}{Scale-RAE}
  \qrow{art}{sefi}{SeFi-Image}
  \qrow{art}{svg}{SVG-T2I}
  \vspace{-\dimexpr\qrowsep+\qcapup\relax}
  \caption{\textbf{Qualitative comparison on WikiArt.} As \cref{fig:supp_qual_coco}, on WikiArt prompts with the WikiArt corpus.}
  \label{fig:supp_qual_art}
  \vspace{\qfigsep}\vfill%
  \qrow{anime}{rae}{Scale-RAE}
  \qrow{anime}{sefi}{SeFi-Image}
  \qrow{anime}{svg}{SVG-T2I}
  \vspace{-\dimexpr\qrowsep+\qcapup\relax}
  \caption{\textbf{Qualitative comparison on Anime.} As \cref{fig:supp_qual_coco}, on Anime prompts with the Anime corpus. Long prompts are shortened to their first sentence.}
  \label{fig:supp_qual_anime}
  \end{minipage}
\end{figure*}
