# Supplementary material for: Retrieval-Seeded Diffusion for Semantic Flow Models
Source: arXiv:2611.39943 source file (2026-11-29)
Supplement: Supplementary file 3 [file fig_supp_qual_coco.tex]

\input{figures/supp_qual/values}%
\begin{figure*}[t]
  \centering
  \input{figures/supp_qual/layout}%
  \qheadrow
  \qrow{coco}{rae}{Scale-RAE}
  \qrow{coco}{sefi}{SeFi-Image}
  \qrow{coco}{svg}{SVG-T2I}
  \vspace{-\dimexpr\qrowsep+\qcapup\relax}
  \caption{\textbf{Qualitative comparison on COCO.} The released sampler with $50$ steps, RMG with $20$ and \method with $8$, from the same noise, on each backbone.}
  \label{fig:supp_qual_coco}
\end{figure*}
