# Supplementary material for: Retrieval-Seeded Diffusion for Semantic Flow Models
Source: arXiv:2611.39943 source file (2026-11-29)
Supplement: Supplementary file 4 [file layout.tex]

\newcommand{\qpanelw}{0.154}%
\newcommand{\qcolsep}{1.5pt}%
\newcommand{\qlabw}{10pt}%
\newcommand{\qpromptsep}{1pt}%
\newcommand{\qrowsep}{2pt}%
\newcommand{\qheadsep}{1pt}%
\newcommand{\qcapup}{3pt}%
\newcommand{\qfigsep}{6pt}%
\newcommand{\qpromptfont}{\scriptsize}%
\newcommand{\qheadfont}{\footnotesize}%
\newcommand{\qlabfont}{\footnotesize}%
\newcommand{\qframe}{0.3pt}%
\definecolor{qbase}{HTML}{EB6834}%
\definecolor{qrmg}{HTML}{4E9F5B}%
\setlength{\fboxsep}{0pt}\setlength{\fboxrule}{\qframe}%
\ifdefined\qtripw\else\newlength{\qtripw}\newlength{\qpw}\fi
\setlength{\qpw}{\qpanelw\linewidth}%
\setlength{\qtripw}{3\qpw}\addtolength{\qtripw}{\qcolsep}\addtolength{\qtripw}{\qcolsep}%
\newcommand{\qv}[1]{\csname suppqual@#1\endcsname}%
\newcommand{\qimg}[2]{\fbox{\includegraphics[width=\dimexpr\qpw-2\fboxrule\relax]{figures/supp_qual/#1/#2.jpg}}}%
\newcommand{\qnone}{\fbox{\parbox[b][\dimexpr\qpw-2\fboxrule\relax][c]{\dimexpr\qpw-2\fboxrule\relax}{\centering\tiny pending}}}%
\newcommand{\qtrip}[3]{\begin{minipage}[b]{\qtripw}\centering
    {\qpromptfont\gridprompt{\qv{#1@#2@#3}}\par}\vspace{\qpromptsep}%
    \ifcsname suppqual@#1@#2@#3@idx\endcsname
      \qimg{#1/#2/\qv{#1@#2@#3@idx}}{base}\hspace{\qcolsep}\qimg{#1/#2/\qv{#1@#2@#3@idx}}{rmg}\hspace{\qcolsep}%
      \qimg{#1/#2/\qv{#1@#2@#3@idx}}{ours}%
    \else\qnone\hspace{\qcolsep}\qnone\hspace{\qcolsep}\qnone\fi
  \end{minipage}}%
\newcommand{\qhead}{\begin{minipage}[b]{\qtripw}\qheadfont
    \parbox[b]{\qpw}{\centering\color{qbase}Baseline}\hspace{\qcolsep}%
    \parbox[b]{\qpw}{\centering\color{qrmg}RMG}\hspace{\qcolsep}%
    \parbox[b]{\qpw}{\centering\color{otherblue}\textbf{\method{} (ours)}}%
  \end{minipage}}%
\newcommand{\qlab}[1]{\parbox[b][\qpw][c]{\qlabw}{\centering\rotatebox{90}{\qlabfont #1}}}%
\newcommand{\qrow}[3]{\noindent\qlab{#3}\hfill\qtrip{#1}{#2}{1}\hfill\qtrip{#1}{#2}{2}\par\vspace{\qrowsep}}%
\newcommand{\qheadrow}{\noindent\hspace*{\qlabw}\hfill\qhead\hfill\qhead\par\vspace{\qheadsep}}%
