# Supplementary material for: Retrieval-Seeded Diffusion for Semantic Flow Models
Source: arXiv:2611.39943 source file (2026-11-29)
Supplement: Supplementary file 5 [file values.tex]

\expandafter\def\csname suppqual@coco@rae@1\endcsname{A red fire hydrant sitting on the side of a road.}%
\expandafter\def\csname suppqual@coco@rae@1@idx\endcsname{p03797}%
\expandafter\def\csname suppqual@coco@rae@2\endcsname{A red and white boat floating along a river.}%
\expandafter\def\csname suppqual@coco@rae@2@idx\endcsname{p02854}%
\expandafter\def\csname suppqual@coco@svg@1\endcsname{A large white clock tower filled with light.}%
\expandafter\def\csname suppqual@coco@svg@1@idx\endcsname{p02552}%
\expandafter\def\csname suppqual@coco@svg@2\endcsname{An elaborate church with tiled floors and stained glass.}%
\expandafter\def\csname suppqual@coco@svg@2@idx\endcsname{p04081}%
\expandafter\def\csname suppqual@coco@sefi@1\endcsname{three dogs on a field of green grass}%
\expandafter\def\csname suppqual@coco@sefi@1@idx\endcsname{p02322}%
\expandafter\def\csname suppqual@coco@sefi@2\endcsname{A man in a suit is wearing a lit up tie.}%
\expandafter\def\csname suppqual@coco@sefi@2@idx\endcsname{p00207}%
\expandafter\def\csname suppqual@anime@rae@1\endcsname{A portrait of a young woman with short, layered blue hair and large blue eyes, wearing a white dress with a blue sash tied at the waist.}%
\expandafter\def\csname suppqual@anime@rae@1@idx\endcsname{p03577}%
\expandafter\def\csname suppqual@anime@rae@2\endcsname{A close-up portrait of a young girl with long, straight white hair, large blue eyes, and a small red hair accessory.}%
\expandafter\def\csname suppqual@anime@rae@2@idx\endcsname{p04964}%
\expandafter\def\csname suppqual@anime@svg@1\endcsname{A close-up portrait of a young girl with bright blonde hair styled in pigtails and large, bright blue eyes.}%
\expandafter\def\csname suppqual@anime@svg@1@idx\endcsname{p03557}%
\expandafter\def\csname suppqual@anime@svg@2\endcsname{A young man with blonde hair, wearing a brown jacket and jeans, sits on the railing of a rooftop overlooking a cityscape during a dramatic sunset.}%
\expandafter\def\csname suppqual@anime@svg@2@idx\endcsname{p04327}%
\expandafter\def\csname suppqual@anime@sefi@1\endcsname{A close-up of a young woman with long, light purple hair, wearing a horned headpiece and a futuristic, metallic headband.}%
\expandafter\def\csname suppqual@anime@sefi@1@idx\endcsname{p02706}%
\expandafter\def\csname suppqual@anime@sefi@2\endcsname{A young woman with large, pointed ears and light brown hair, wearing a purple dress, a dark vest, and metallic arm and leg armor.}%
\expandafter\def\csname suppqual@anime@sefi@2@idx\endcsname{p03217}%
\expandafter\def\csname suppqual@art@rae@1\endcsname{A painting of a cliff overlooking the ocean, with a small boat in the distance and a cloudy sky above.}%
\expandafter\def\csname suppqual@art@rae@1@idx\endcsname{p03656}%
\expandafter\def\csname suppqual@art@rae@2\endcsname{A black and white sketch of trees and bushes, rendered in an impressionistic style.}%
\expandafter\def\csname suppqual@art@rae@2@idx\endcsname{p04640}%
\expandafter\def\csname suppqual@art@svg@1\endcsname{A painting of a mountain view with a vase of white flowers in the foreground.}%
\expandafter\def\csname suppqual@art@svg@1@idx\endcsname{p01685}%
\expandafter\def\csname suppqual@art@svg@2\endcsname{A cowboy sits on a rock, gazing up at the night sky.}%
\expandafter\def\csname suppqual@art@svg@2@idx\endcsname{p00216}%
\expandafter\def\csname suppqual@art@sefi@1\endcsname{A painting of a bird and a lion with a dark background.}%
\expandafter\def\csname suppqual@art@sefi@1@idx\endcsname{p01937}%
\expandafter\def\csname suppqual@art@sefi@2\endcsname{A painting of three children on a beach, with one child in a white dress and two in white dresses, holding hands and walking towards the water.}%
\expandafter\def\csname suppqual@art@sefi@2@idx\endcsname{p04867}%
