# Supplementary material for: Retrieval-Seeded Diffusion for Semantic Flow Models
Source: arXiv:2611.39943 source file (2026-11-29)
Supplement: Supplementary file 6 [file A_additional.tex]

\section{Additional results}
\label{app:results}
\subsection{Store sizes and latency}
\label{app:cost}
\paragraph{Store sizes.}
\Cref{tab:store_size} gives the exact size of every store. The fp16 latents of each corpus in each
backbone's latent space, of which a prompt reads $k$ rows, and the SigLIP-2 keys which the search
reads in full and which all three backbones share.

\paragraph{Latency.}
\Cref{tab:latency} times one prompt at batch size $1$ on one GPU, as the median over $100$ prompts for
the read and over $20$ for sampling ($10$ on SeFi-Image). The one-time read includes the SigLIP-2 embedding of the prompt,
the exact search over the shared keys and the read of the
$k = 50$ latents of \method or the $20$ of RMG's bank, done once per prompt. It takes $2$ to $7$\,ms,
against $32$ to $37$\,ms for one forward pass of Scale-RAE or SVG-T2I.
Sampling time is the wall-clock time to generate one image without the backbone's text encoder and decoder,
which every sampler runs once per image. It covers the denoising steps and for RMG and \method the one-time read too.
On Scale-RAE, a guided step of \method and RMG
runs its two passes one after the other. \method is $3.15\times$ faster than the released sampler on
Scale-RAE, close to its $3.125\times$ fewer network evaluations, and
$6.24\times$ and $6.23\times$ faster on SVG-T2I and SeFi-Image, close to its $6.25\times$ fewer
steps. RMG, with $20$ guided steps, is $1.23\times$, $2.50\times$ and $2.51\times$ faster than the
released sampler, so \method is $2.5$ to $2.6\times$ faster than RMG on all three.
SeFi-Image's text encoder and decoder are not timed separately, so we take its step as the
time difference between $50$ and $8$ steps of its released sampler divided by $42$.

\subsection{Equal step counts}
\label{app:prdc}
\Cref{tab:main} compares methods at their default settings. Here
Gaussian sampling, RMG and \method run at the same number of steps, from $4$ to $50$, on COCO
(\cref{fig:fid_vs_nfe,tab:app_prdc}).

\method has a lower FID than Gaussian sampling at every step count on all three backbones, so its
gain does not come from taking fewer steps. More steps change little for either. From $8$ to $50$
steps Gaussian sampling gains at most $1.4$ FID and \method moves by at most $1.3$, so comparing
against the released samplers at $50$ steps does not handicap them. The exception is SeFi-Image
which is $2.0$ points better at its $8$ steps point and there \method at $8$ steps still beats it, $31.60$ against
$35.32$.
On Scale-RAE the released sampler is unguided ($w=1$), so at the same step count
\method makes twice its network evaluations. Guidance does not help the released sampler, whose FID
at $w = 4$ and $50$ steps rises to $32.53$ (\cref{tab:guidance}).
\input{tables/store_size/tab_store_size}
\input{tables/latency/tab_latency}
\input{tables/app_prdc/app_prdc}
\input{figures/fid_vs_nfe/fid_vs_nfe}

One might wonder if \method buys its FID by dropping modes, which would lower recall and coverage but it does not.
Both are higher than Gaussian sampling's at every step count on all three backbones. Precision and density
are higher at every step count on SVG-T2I, and on Scale-RAE and SeFi-Image they are either higher or
within $0.025$ of Gaussian sampling's.
\newpage

\subsection{Another solver}
\label{app:solver}
\Cref{tab:solver} repeats the comparison at $N = 8$ with DPM-Solver++(2M)~\cite{lu2022dpmsolverpp}, a
second-order multistep solver that makes one network call per step on the same time grid.
It lowers FID by $0.2$ to $0.8$ for both Gaussian sampling and \method, and \method's gain over Gaussian sampling
barely changes - $9.2$ and $9.1$ FID points on Scale-RAE with Euler and DPM-Solver++, $6.8$ and $6.5$
on SVG-T2I, and $3.7$ and $3.9$ on SeFi-Image.
\input{tables/solver/tab_solver}

\subsection{Memorisation audit}
\label{app:memorization}
\input{figures/t0_line/fig_t0_line}
\input{tables/memorization/memorization}
\input{tables/fd_cmmd/fd_cmmd}

An anchor drawn from real images invites the question of whether the output is one of the retrieved images~\cite{carlini2023extracting,somepalli2023diffusion}.
Copying would pay off in FID. Decoding the nearest retrieved latent with no generation at all
scores $14.03$ on Scale-RAE and $14.35$ on SVG-T2I. We
score the maximum similarity of every generation to the whole corpus with SSCD~\cite{pizzi2022self}
and read it against the real held-out image
belonging to each prompt, scored the same way. \vadjust{\vfill\penalty-10000\null\vfill\penalty-10000}%
SSCD is an image descriptor trained for copy detection, so an image and its edited copies (cropped, recoloured, overlaid) get close descriptors and two images are compared by their cosine similarity.

The Held-out images are the informative part of \cref{tab:memorization}. Held-out images exceed the
conventional copy threshold of $0.5$~\cite{somepalli2023diffusion} for $3.82$ to $6.00\%$ of
prompts, because real images of the same subject resemble each other. \method stays at or below
$0.32\%$ in all nine settings and at most $0.16$ points above
the released sampler's. RMG reaches $1.10\%$ on Scale-RAE on Anime. Moving the start further along the
path raises the rate above the released sampler's from $t_0 = 0.1$ (\cref{fig:t0_line}).

\subsection{\texorpdfstring{FD$_\text{DINOv2}$}{FD-DINOv2} and CMMD}
\label{app:fd_cmmd}
\input{tables/rmg_k20/tab_rmg_k20}
FID and KID compare Inception features, which can disagree with human judgement on modern
generators~\cite{stein2023exposing,jayasumana2024rethinking}. \Cref{tab:fd_cmmd} repeats the comparison
of \cref{tab:main} in two other feature spaces, against the same held-out images.
FD$_\text{DINOv2}$~\cite{stein2023exposing} is the Fr\'echet distance between DINOv2 ViT-L/14 features,
and CMMD~\cite{jayasumana2024rethinking} is the maximum mean discrepancy between CLIP ViT-L/14
embeddings under a Gaussian kernel of bandwidth $10$, reported $\times 10^3$ as in its reference
implementation. \method has the lowest FD$_\text{DINOv2}$ in all nine settings and the lowest CMMD in
eight. The exception is SeFi-Image on COCO, where the released sampler and RMG reach a lower CMMD,
$0.559$ and $0.579$ against $0.602$. SeFi-Image generates in a space built on DINOv2 features, where its anchor is also computed,
so on SeFi-Image CMMD is the more independent of the two.

\subsection{RMG at the same \texorpdfstring{$k$}{k}}
\label{app:rmg}
\Cref{tab:main} gives \method $k = 50$ neighbours and RMG a bank of $20$, the bank size of their
paper. \Cref{tab:app_rmg} removes that difference and lets both methods read the same $k$ images that our
search returns for each COCO val2017 prompt, at $k = 20$ and at $k = 50$. Each method is at its own number of
steps, $8$ for \method and $20$ for RMG.

At both values of $k$, \method has the lowest FID and KID on Scale-RAE and SVG-T2I and higher diversity than
RMG on almost all metrics, while RMG keeps the higher CLIP on Scale-RAE. On SeFi-Image the two are
almost level in FID and KID while RMG has slightly higher diversity and \method has slightly higher CLIP.
From $k = 20$ to $k = 50$ the FID of \method moves by at most $0.11$.

\subsection{Per-prompt diversity}
\label{app:diversity}
\Cref{fig:diversity_bars} shows the per-prompt diversity on COCO discussed in \cref{sec:exp:diversity},
\method and RMG at their default settings, each reported as the change from its backbone's released sampler. \Cref{fig:div_grid} shows four samples per prompt from each method.

\input{figures/diversity_bars/fig_diversity_bars}
\input{figures/div_grid/fig_div_grid}%
