# Supplementary material for: Retrieval-Seeded Diffusion for Semantic Flow Models
Source: arXiv:2611.39943 source file (2026-11-29)
Supplement: Supplementary file 7 [file suppl.tex]

\clearpage
\maketitlesupplementary

\makeatletter
\newcommand{\suppclearpage}{\clearpage\global\@colroom\@colht\global\vsize\@colht
  \global\@toproom\topfraction\@colht\global\@botroom\bottomfraction\@colht}
\makeatother
\makeatletter
\setlength{\@fptop}{0pt}\setlength{\@fpsep}{\floatsep}\setlength{\@fpbot}{0pt plus 1fil}%
\setlength{\@dblfptop}{0pt}\setlength{\@dblfpsep}{\dblfloatsep}\setlength{\@dblfpbot}{0pt plus 1fil}%
\makeatother
\renewcommand{\thesection}{\Alph{section}}
\setcounter{section}{0}
\renewcommand{\theHsection}{app.\arabic{section}}
This supplementary material adds to the main paper.

\Cref{app:results} gives the further results that the main paper leaves out: store sizes and latency, the comparison at equal step counts and with
another solver, the memorisation audit, two more feature space metrics, RMG at the same $k$, and
per-prompt diversity.
\Cref{app:setup} gives the implementation details: backbones, retrieval, RMG and metrics.
\Cref{app:qual} shows more qualitative results on all three datasets.
\Cref{app:ablations} gives the ablations behind our default settings.
\Cref{app:anchor} shows different anchors and noise.
\Cref{app:limitations} lists the limitations.

\input{sections/app/A_additional}

\suppclearpage
\input{sections/app/B_implementation}

\input{sections/app/C_qualitative}

\suppclearpage\suppressfloats[t]
\input{sections/app/D_ablations}

\suppclearpage
\input{sections/app/E_anchor}

\newpage
\input{sections/app/F_limitations}
